# Supplementary material for: Polyhedral Clinching Auctions and the Adwords Polytope
Source: arXiv:1201.0404 source file (2012-05-18)
Supplement: Supplementary file 1 [file budgets-appendix.tex]

\section{Non-convexity of Pareto-\columnsversion{}{\\}optimal
mechanisms}\label{appendix:non_convex}

Here we discuss
the point made in Section \ref{sec:setting_polyhedral_clinching} that the set
of Pareto-optimal mechanisms is not convex. Consider the environment $P = \{x
\in \R^2_+; x_1 + x_2 \leq 1\}$ studied in \cite{dobzinski_budgets}. Notice
that this environment is nice, in the sense that the set of undominated
allocations is a convex set. 
For fixed budgets $B_1 \geq B_2$, the following is a mechanism with all the desirable
properties:

\columnsversion{
$$x^{B_1,B_2}(v_1, v_2) = \left\{
\begin{aligned}
&(0,1), & v_2 \geq v_1, v_1 \leq B_2 \\
& (1-\frac{B_2}{v_1},\frac{B_2}{v_1}),&v_2 \geq v_1, B_2 \leq v_1 \leq B_1\\
& (1-\frac{1}{2} \frac{B_2}{B_1}\left[ 1+\frac{B_1^2}{v_1^2} \right],\frac{1}{2}
\frac{B_2}{B_1}\left[ 1+\frac{B_1^2}{v_1^2} \right]),&v_2 \geq v_1, v_1 \geq
B_1\\
&(1,0), & v_1 > v_2, v_2 \leq B_1 \\
& (1+\frac{1}{2} \frac{B_2}{B_1}\left[-1+\frac{B_1^2}{v_2^2}
\right],\frac{1}{2} \frac{B_2}{B_1}\left[1-\frac{B_1^2}{v_2^2} \right] ),&v_1
> v_2, v_2 \geq B_1\\
\end{aligned}
\right.$$}{

$$\begin{aligned}
& x^{B_1,B_2}(v_1, v_2) = \\
& \left\{
\begin{aligned}
&(0,1), v_2 \geq v_1, v_1 \leq B_2 \\
& (1-\frac{B_2}{v_1},\frac{B_2}{v_1}),v_2 \geq v_1, B_2 \leq v_1 \leq B_1\\
& (1-\frac{1}{2} \frac{B_2}{B_1}\left[ 1+\frac{B_1^2}{v_1^2} \right],\frac{1}{2}
\frac{B_2}{B_1}\left[ 1+\frac{B_1^2}{v_1^2} \right]),v_2 \geq v_1, v_1 \geq
B_1\\
&(1,0),  v_1 > v_2, v_2 \leq B_1 \\
& (1+\frac{1}{2} \frac{B_2}{B_1}\left[-1+\frac{B_1^2}{v_2^2}
\right],\frac{1}{2} \frac{B_2}{B_1}\left[1-\frac{B_1^2}{v_2^2} \right] ),v_1
> v_2, v_2 \geq B_1\\
\end{aligned}
\right. \end{aligned}$$
}

Now, consider the mechanism defined by $\tilde{x} = \frac{1}{2} x^{B_1, B_2}
+\frac{1}{2} x^{B'_1, B'_2}$. This mechanism is clearly truthful (since
truthfulness is a linear property), and the payments of the corresponding
payment rule are such that $\tilde{p}_i \leq \tilde{B}_i := \frac{1}{2} B_i +
\frac{1}{2} B'_i $ and all goods are allocated, in the sense that
$\tilde{x}_1(v) + \tilde{x}_2(v)= 1$. However, it is \emph{not} the case that
it is Pareto optimal for budgets $\tilde{B}_1,\tilde{B}_2$.

Consider for example $B_1 = B'_1 = 3, B_2 = 2, B'_2 = 1$, then consider the
mechanism $\tilde{x} = \frac{1}{2} x^{B_1, B_2}
+\frac{1}{2} x^{B'_1, B'_2}$ for budgets $\tilde{B}_1 = 3, \tilde{B}_2 = 1.5$
and consider some $v_1, 1<v_1<1.5$, now, note that $\lim_{v_2 \rightarrow \infty}
x_2(v_1, v_2) < 1$ but the budget never gets exhausted, which contradicts
Lemma \ref{charac-lemma}.

\comment{

\begin{proof}
 If $x \in P^*$, then clearly $x(S) \leq f^*(S), \forall S$. Now, for the
other direction, suppose the vector $\hat{x}$ is such that $\hat{x}(S) \leq
f^*(S), \forall S$. We need to show that there exists $x_i^j$ such that:
\begin{equation}\label{hall-primal}
\begin{aligned}
& \sum_{j \in \Gamma(i)} x_i^j = \hat{x}_i, & \forall i \\
& \sum_{i \in S} x_i^j \leq f_j(S), &\forall S \subseteq \Gamma(j) \\
& x_i^j \geq 0, & \forall i,j
\end{aligned}
\end{equation}
Showing that the program (\ref{hall-primal}) is feasible is equivalent to
showing that the solution of the dual program (\ref{hall-dual}) is bounded,
which is the same as all the feasible points having non-negative objective:
\begin{equation}\label{hall-dual}
\begin{aligned}
& \min \sum_i y_i \hat{x}_i + \sum_{j, S \subseteq \Gamma(j)} z_S^j f_j(S)
\qquad \text{s.t.} \\
& y_i + \sum_{S \subseteq \Gamma(j), S \ni i} z_S^j \geq 0, & \forall j \in
\Gamma(i) \\
& z_S^j \geq 0
\end{aligned}
\end{equation}
This is equivalent to proving that for all $z_S^j \geq 0$, the following is
true:
\begin{equation}\label{goal-lemma-3}
-\sum_i \hat{x}_i \left( \min_{j \in \Gamma(i)} \sum_{S; i\in S \subseteq
\Gamma(j) } z_S^j  \right) + \sum_{j, S \subseteq  \Gamma(j)}  f_j(S) z_S^j
\geq 0
\end{equation}

To show this fact, define $\chi(i) = \min_{j \in \Gamma(i)} \sum_{S; i\in S
\subseteq \Gamma(j)} z_S^j $. Wlog we can assume that $\chi(1) \geq \chi(2) 
\geq \hdots \chi(n)$. Given that, we can rewrite:
$$\sum_i \hat{x}_i \chi(i) = \sum_i (\chi(i) - \chi(i+1)) \sum_{t \leq i}
\hat{x}_t \leq \sum_i (\chi(i) - \chi(i+1)) \sum_j f_j(\{1..i\} \cap \Gamma(j))
$$
To show (\ref{goal-lemma-3}), we will show that for each $j$:
$$\sum_i (\chi(i) - \chi(i+1)) f_j(\{1..i\} \cap \Gamma(j)) \leq  \sum_{S
\subseteq  \Gamma(j)}  f_j(S) z_S^j$$
We do so by rewriting the equation above in terms of the marginals:
$$\sum_i (\chi(i) - \chi(i+1)) \sum_{t \in \{1..i\} \cap \Gamma(j) }
f_j(t \vert \{1..t-1\} \cap \Gamma(j)) \leq \sum_{S
\subseteq  \Gamma(j)}   z_S^j \sum_{t \in S} f_j(t \vert \{1..t-1\} \cap S)$$
where $f(i \vert S) = f(S \cup i) - f(S)$.
Now, we invoke submodularity to see that for $S \subseteq \Gamma(j)$, $f_j(t
\vert \{1..t-1\} \cap S) \geq f_j(t \vert \{1..t-1\} \cap \Gamma(j))$. Now,
after applying this inequality, compare the coefficients of $f_j(t \vert
\{1..t-1\} \cap \Gamma(j))$ in each of the sides. In the left side, the
coefficient is $\chi(t)$ and for the right side, the coefficient is $\sum_{S
\subseteq \Gamma(j), t \in S} z_S^j$. Now, by the definition of $\chi$,
$\chi(t) \leq \sum_{S \subseteq \Gamma(j), t \in S} z_S^j$, 
and the proof is complete.
\end{proof}

}
